# Supplementary material for: The INPOP10a planetary ephemeris and its applications in fundamental physics
Source: arXiv:1108.5546 source file (2011-08-29)
Supplement: Supplementary file 1 [file fienga_supp2.pdf]

Online Resource 3 to the paper "The INPOP10a planetary ephemeris and its applications in fundamental physics." by Fienga[1] et al. published in Cel. Mech. and Dyn. Astr.

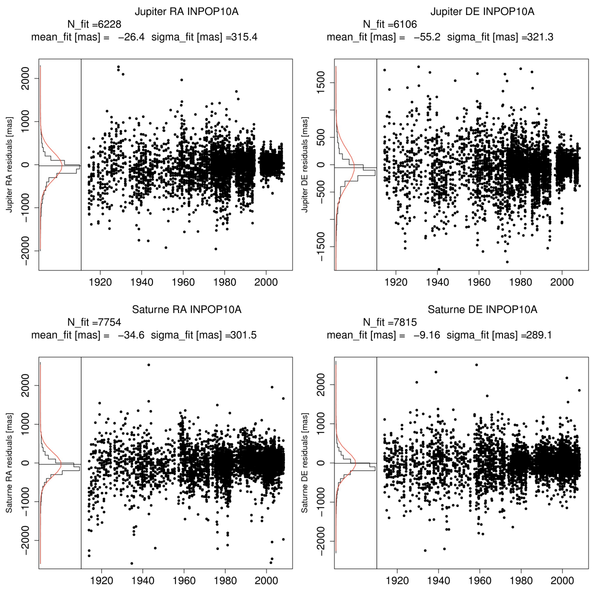


**Fig. 1** Optical residuals of Jupiter in right ascension (line 1) and declination (line 2) and of Saturne (lines 3 and 4) based on INPOP06 (left-hand side), INPOP08 (middle) and INPOP10a (right-hand side). Light colors stand for extrapolated residuals.

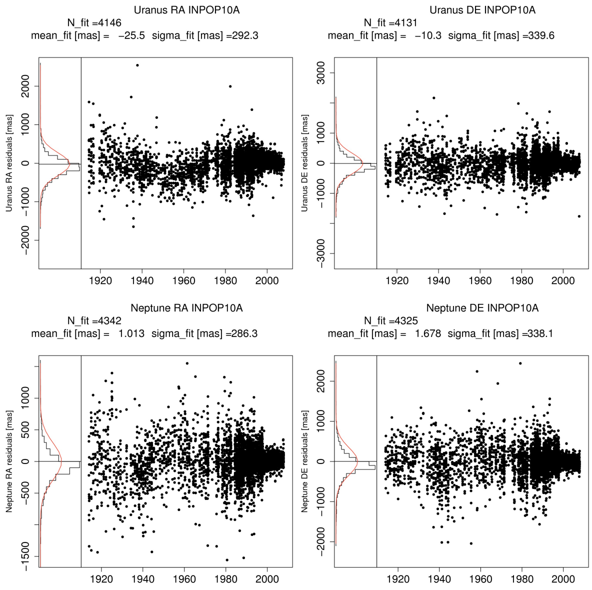


**Fig. 2** Optical residuals of Uranus in right ascension (line 1) and declination (line 2) and of Neptune (lines 3 and 4) based on INPOP06 (left-hand side), INPOP08 (middle) and INPOP10a (right-hand side). Light colors stand for extrapolated residuals.

E-mail: agnes.fienga@obs-besancon.fr

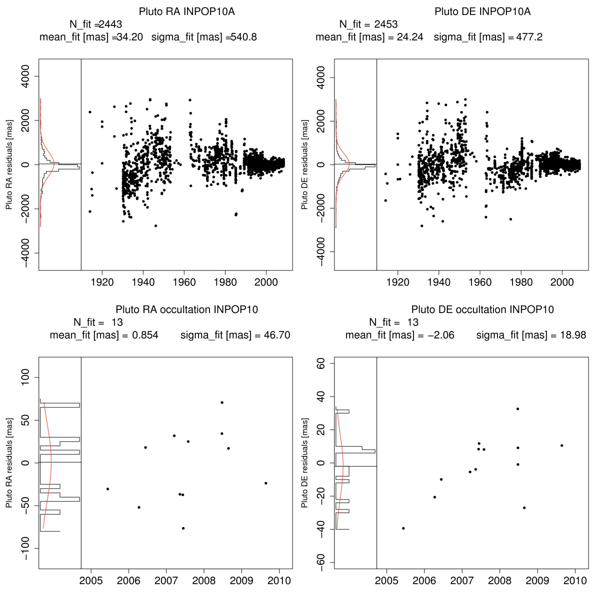


**Fig. 3** Pluto residuals in right ascension (lines 1 and 3) and declination (lines 2 and 4) deduced from optical observations (lines 1 and 2) and stellar occultations (lines 3 and 4) based on INPOP06 (left-hand side), INPOP08 (middle) and INPOP10a (right-hand side). Light colors stand for extrapolated residuals.

E-mail: agnes.fienga@obs-besancon.fr
