# Supplementary material for: The INPOP10a planetary ephemeris and its applications in fundamental physics
Source: arXiv:1108.5546 source file (2011-08-29)
Supplement: Supplementary file 2 [file fienga_supp3.pdf]

Online Resource 2 to the paper "The INPOP10a planetary ephemeris and its applications in fundamental physics." by Fienga[1] et al. published in Cel. Mech. and Dyn. Astr.

---

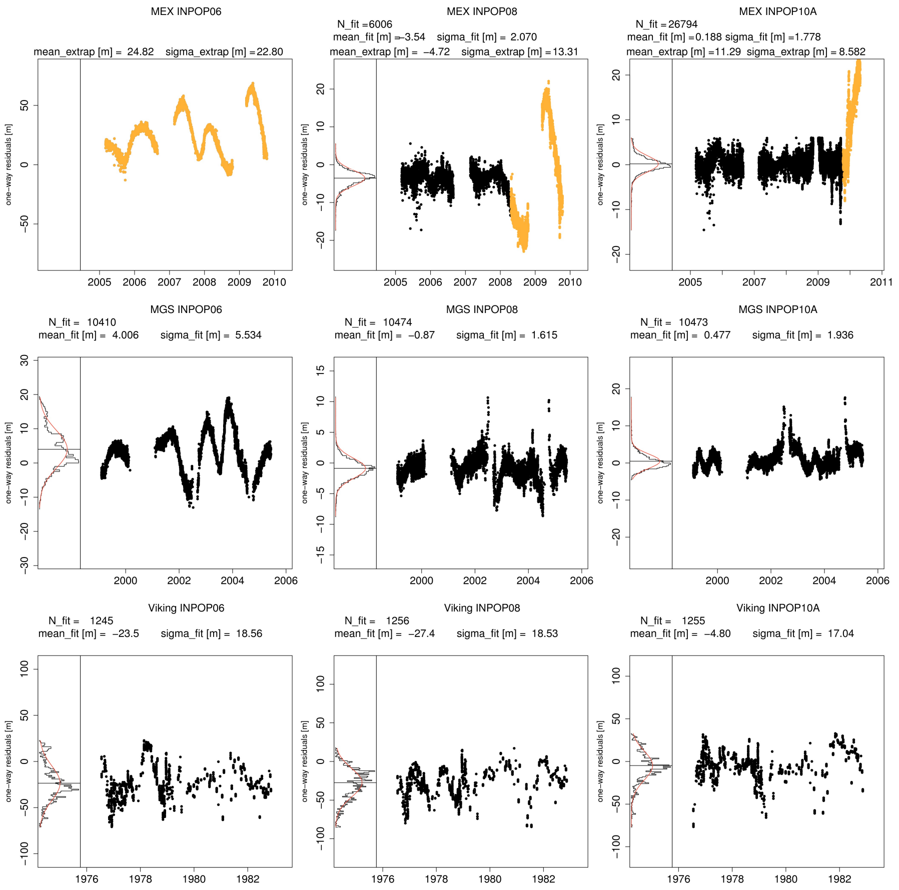


**Fig. 1** MEX (line 1), MGS (line 2) and Viking (line 3) residuals based on INPOP06 (left-hand side), INPOP08 (middle) and INPOP10a (right-hand side). Light colors stand for extrapolated residuals.

E-mail: agnes.fienga@obs-besancon.fr

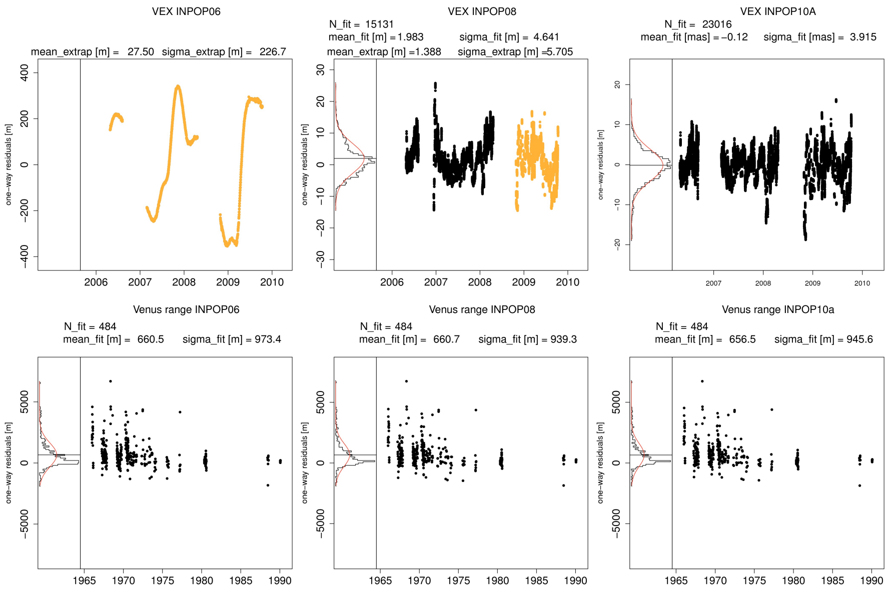


**Fig. 2** VEX (line 1) residuals based on INPOP06 (left-hand side), INPOP08 (middle) and INPOP10a (right-hand side). Light colors stand for extrapolated residuals.

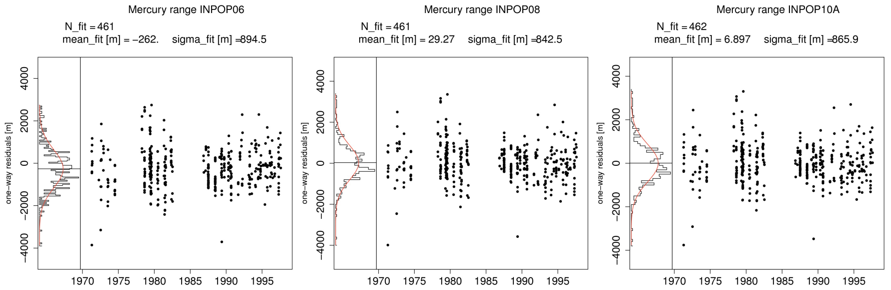


**Fig. 3** Mercure (line 1) residuals based on INPOP06 (left-hand side), INPOP08 (middle) and INPOP10a (right-hand side). Light colors stand for extrapolated residuals.

E-mail: agnes.fienga@obs-besancon.fr

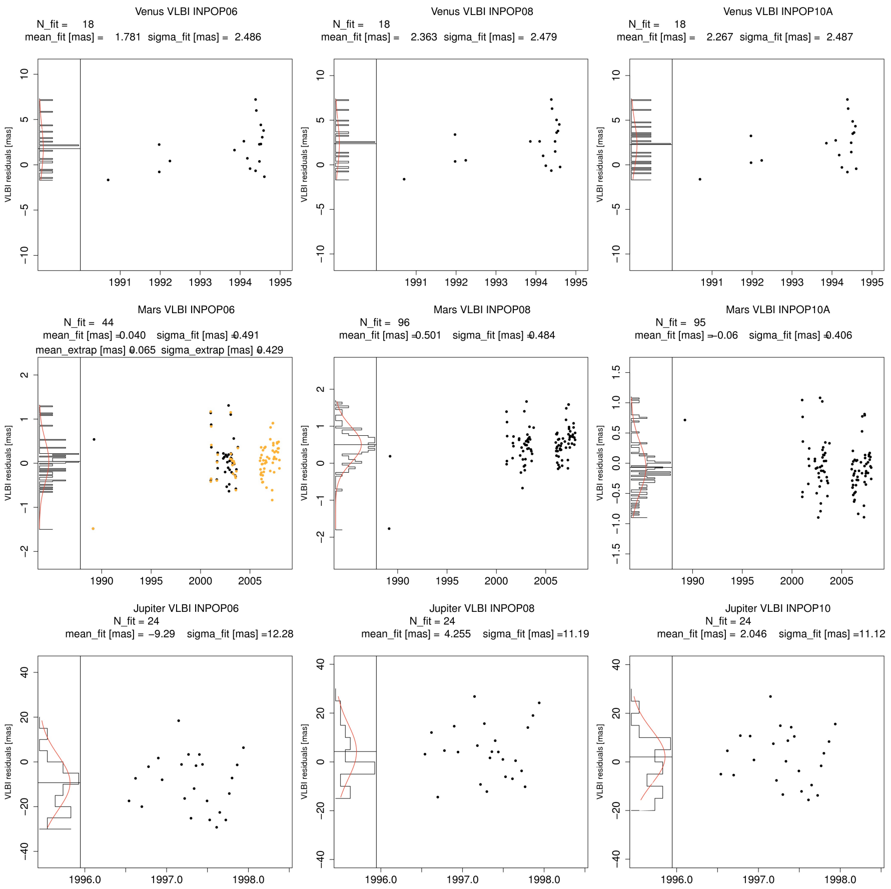


**Fig. 4** VLBI de Venus (line 1), Mars (line 2) and Jupiter (line 3) residuals based on INPOP06 (left-hand side), INPOP08 (middle) and INPOP10a (right-hand side). Light colors stand for extrapolated residuals.

E-mail: agnes.fienga@obs-besancon.fr

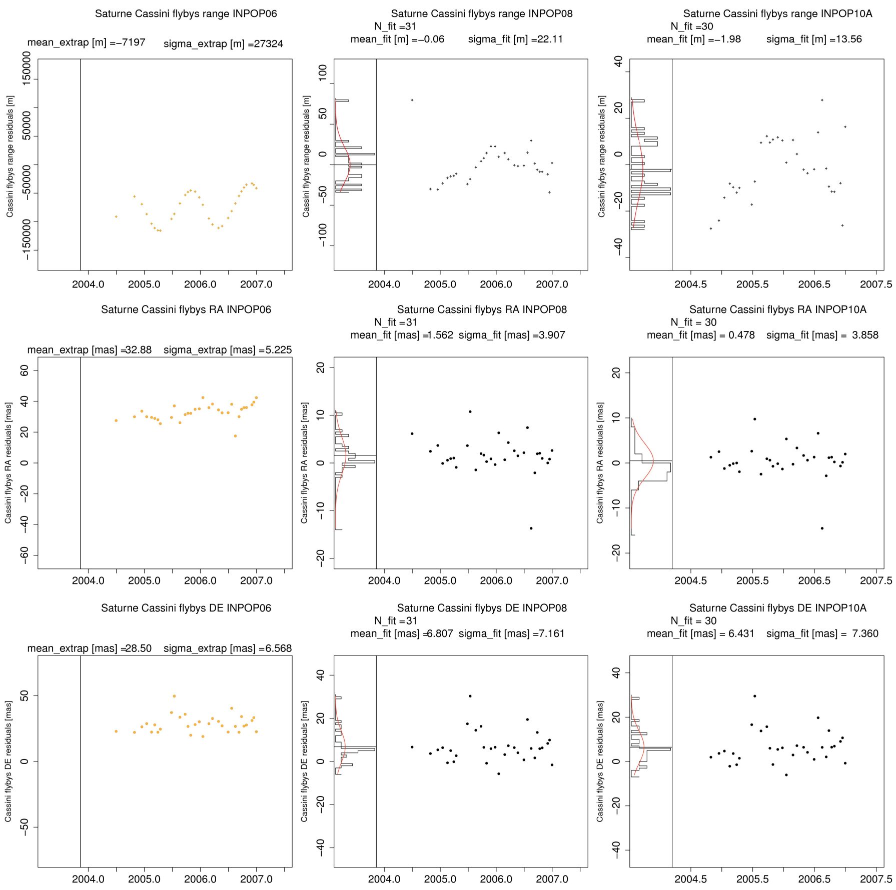


**Fig. 5** Cassini tracking residuals based on INPOP06 (left-hand side), INPOP08 (middle) and INPOP10a (right-hand side) given in right ascension (line 3), declination (line 2) and geocentric distances (line 1). Light colors stand for extrapolated residuals.

E-mail: agnes.fienga@obs-besancon.fr

Online Resource 2 to the paper "The INPOP10a planetary ephemeris and its applications in fundamental physics." by Fienga[1] et al. published in Cel. Mech. and Dyn. Astr.

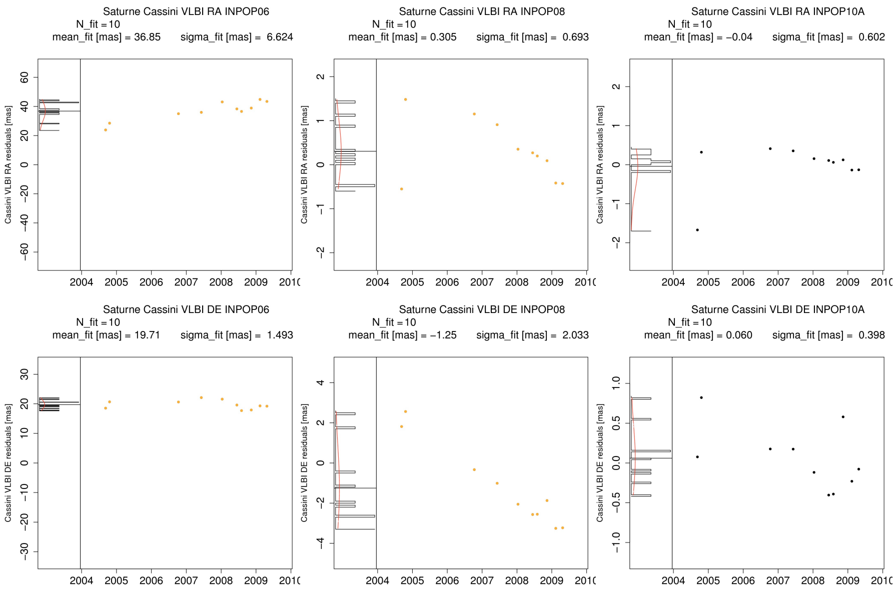


**Fig. 6** Cassini VLBI residuals based on INPOP06 (left-hand side), INPOP08 (middle) and INPOP10a (right-hand side) given in right ascension (line 3) and declination (line 2). Light colors stand for extrapolated residuals.

E-mail: agnes.fienga@obs-besancon.fr
